# Supplementary material for: An Orientation Bias in Observations of Submillimetre Galaxies
Source: arXiv:2106.11588 source file (2022-08-30)
Supplement: Supplementary file 1 [file appendix.tex]

\section{Measuring and sampling from the dimming distribution}
\label{sec:sampling}

\begin{figure}
	\includegraphics[width=\columnwidth]{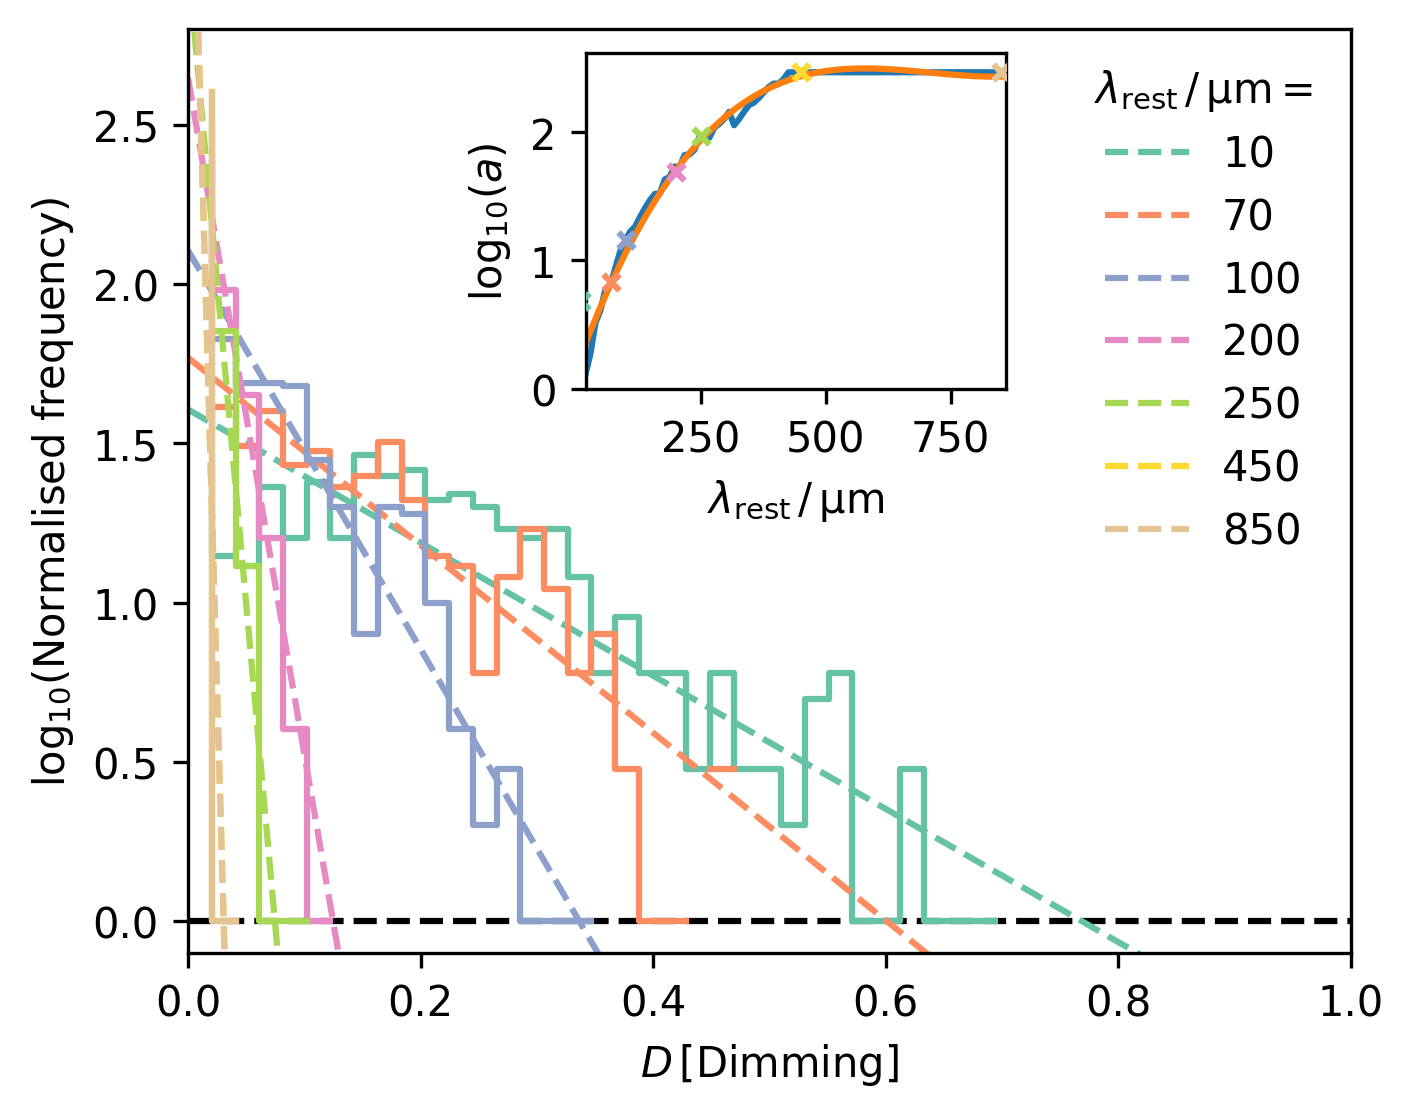}
    \caption{Binned distribution of dimming fraction for all galaxies and orientations combined (solid) at four different wavelengths, with fits (dashed).
    }
    \label{fig:dimming_distribution}
\end{figure}

For each orientation $i \in [n]$ of each simulated galaxy $g$, where $n = \{1, \cdots, 50\}$, we calculated the normalised emission at wavelength $\lambda$,
\begin{equation}
  D^{i}_{g} = 1 - \frac{S^{i}_{g}(\lambda)}{\max\limits_{i \in n} \, S^{i}_{g}(\lambda)} \;\;,
\end{equation}
where $D$ can be considered the relative dimming.
\fig{dimming_distribution} shows the distribution of $D$ for all galaxies and orientations combined, at four different wavelengths.
This distribution can be approximated by
\begin{equation}
  1 - D = \frac{e^{ax - 1}}{b} \;\;,
\end{equation}
where $a$ is analogous to the rate parameter in the exponential distribution, and $b$ sets the normalisation.
Fits to the stacked distribution from our simulated galaxy sample give $a = 9.58$ (at 250 \mumetre, observer-frame).

To sample from this distribution we used inverse transform sampling; we first transformed $D$ to a probability density function, integrated to obtain the cumulative distribution function (CDF), and then found the inverse to give $D_{g}$, the estimated dimming for each randomly sampled galaxy $g$,
\begin{equation}
  D_{g} = 1 - \frac{\mathrm{log} \left( x (e^{a - 1} - e^{-1}) \right)}{a} \;\;,
\end{equation}
where $x$ is a random variable sampled from the uniform distribution $U(0,1)$.
